# Supplementary material for: Tracking Any Point with Agentic Visual Reasoning
Source: arXiv:2611.34943 source file (2026-11-25)
Supplement: Supplementary file 1 [file supplement_contents.tex]

\noindent\begin{minipage}{\linewidth}
\normalfont\normalsize
\color{black}
\hypersetup{linkcolor=black}
\setlength{\parskip}{0pt}
\setlength{\parindent}{0pt}
\makeatletter
\let\texorpdfstring\@secondoftwo
\def\@pnumwidth{2.2em}
\def\@tocrmarg{3.2em}
\newcommand{\suppcontentsgroup}[1]{%
  \par\vspace{9pt}\noindent
  \hyperref[#1]{\textcolor{suppheading}{\textbf{\ref*{#1}\ \nameref*{#1}}}}%
  \hfill\hyperref[#1]{\textbf{\pageref*{#1}}}\par\vspace{2pt}}
\newcommand{\suppcontentsentry}[1]{%
  \@dottedtocline{1}{1em}{2.6em}%
    {\hyperref[#1]{\numberline{\ref*{#1}.}\nameref*{#1}}}%
    {\hyperref[#1]{\pageref*{#1}}}}
{\large\bfseries Contents}\par\vspace{2pt}
\suppcontentsgroup{sec:supp-trackingbench}
\suppcontentsentry{sec:supp-video-selection}
\suppcontentsentry{sec:supp-query-pool}
\suppcontentsentry{sec:supp-benchmark-composition}
\suppcontentsentry{sec:supp-heldout-annotation}
\suppcontentsentry{sec:supp-evaluation-protocol}
\suppcontentsgroup{sec:supp-agentap}
\suppcontentsentry{sec:supp-tool-interface}
\suppcontentsentry{sec:supp-inference-protocol}
\suppcontentsentry{sec:supp-agent-settings}
\suppcontentsentry{sec:supp-runtime-cost}
\suppcontentsentry{sec:supp-example-sessions}
\suppcontentsgroup{sec:supp-results}
\suppcontentsentry{sec:supp-complete-results}
\suppcontentsentry{sec:supp-localization-reappearance}
\suppcontentsentry{sec:supp-agent-ablations}
\suppcontentsentry{sec:supp-scaling}
\suppcontentsentry{sec:supp-qualitative}
\suppcontentsgroup{sec:supp-egotap4d}
\suppcontentsentry{sec:supp-recordings}
\suppcontentsentry{sec:supp-trajectory-annotation}
\suppcontentsentry{sec:supp-annotation-quality}
\suppcontentsentry{sec:supp-d4rt}
\makeatother
\end{minipage}\par\vspace{10pt}
